# Supplementary material for: PAN: A World Model for General, Actionable, and Long-Horizon World Simulation
Source: arXiv:2511.09057 source file (2026-09-05)
Supplement: Supplementary file 1 [file appendix.tex]

% Authors may wish to optionally include extra information (complete proofs, additional experiments and plots) in the appendix. All such materials should be part of the supplemental material (submitted separately) and should NOT be included in the main submission.
\clearpage
\section{Data Processing}
\subsection{Data Filtering}
As mentioned in \ref{sec:instruction_tuning_data}, we adopt some filtering policy to eliminate undesirable video data:
\begin{itemize}
    \item \textbf{Low-quality video}: To remove low-quality video, we use an image aesthetic predictor\footnote{\url{https://github.com/christophschuhmann/improved-aesthetic-predictor}} to predict the aesthetic score. Specifically, for each video clip, we select three equidistant frames and average their aesthetic scores to determine the video’s overall aesthetic score. We then filter out video clips with an aesthetic score lower than 4.5.
    \item \textbf{Static video}: To avoid videos with relatively static scenes, we calculate the optical flow magnitude (OFM) for each video clip and filter out those with an OFM lower than 2.0.
    \item \textbf{Edited video}: Since lots of videos in Panda-70M contain edited scenes, which can harm the model's generative abilities, we detect these by evaluating the edge intensity and luminance distribution of the video clips. Specifically, we use SceneDetect\footnote{\url{https://www.scenedetect.com/}} to assess both edge intensity (\texttt{delta\_edges}) and luminance distribution (\texttt{delta\_lum}).
    \item \textbf{Overlong/overshort video}: We focus on videos with a length between 1 and 10 seconds, filtering out those that are either too long or too short.
\end{itemize}
After obtaining the desired videos, we split each video into multiple clips (1-3 clips) with randomly sampled FPS. We then generate captions using GPT-4 Turbo.

\subsection{Data Captioning}

The open-source video-text datasets available in the community do not align with our goals, necessitating re-annotation of the videos. Since human annotation is both costly and time-consuming, we use GPT-4 Turbo to re-caption the videos. Specifically, for each video clip, we sample 4 frames to provide GPT-4 Turbo with sequential information about the video. The prompt we use are given below:
\begin{itemize}
    \item \textbf{Single clip}: \texttt{You are given a series of continuous frames. Identify and describe the new information appearing in the frames. New information refers to details not discernible from previous frames. This includes human actions, the appearance of new objects, or changes in the scene. For human-related content, provide specific descriptions, such as 'a person talks while looking down', instead of just stating 'talking'. If no humans are present, avoid assuming or creating human actions. Include details of scene changes or new objects that appear. Aim for precision in your descriptions. If no significant actions or new objects are visible, describe any notable camera movements. Avoid using directional terms like 'left' and 'right'. Provide the observations in a caption. The caption should be detailed, containing approximately five sentences that cover the actions of the main and secondary subjects, any new subjects or objects, and any changes in camera movement. Refrain from using subjective interpretations such as 'indicating' or 'suggesting', and avoid starting phrases like 'as the frames progress'. Directly generate factual and observational captions without introductory phrases like 'In the frames:' or 'In the video'  .The captions should be useful for text-to-video generation task. }
    \item \textbf{Two clips}: \texttt{You are given a series of continuous frames divided into 2 segments. Identify and describe the new information appearing in each segment. New information refers to details not discernible from previous frames. This includes human actions, the appearance of new objects, or changes in the scene. For human-related content, provide specific descriptions, such as 'a person talks while looking down', instead of just stating 'talking'. If no humans are present, avoid assuming or creating human actions. Include details of scene changes or new objects that appear. Aim for precision in your descriptions. If no significant actions or new objects are visible, describe any notable camera movements. Avoid using directional terms like 'left' and 'right'. Provide the observations in 2 separate captions divided by a '\#'. Each caption should be detailed, containing approximately five sentences that cover the actions of the main and secondary subjects, any new subjects or objects, and any changes in camera movement. Refrain from using subjective interpretations such as 'indicating' or 'suggesting', and avoid starting phrases like 'as the frames progress'. Directly generate factual and observational captions without introductory phrases like 'Segment 1:' or 'In this/first/second segment'. The captions should be useful for text-to-video generation task. Avoid to generate 'the first/second/third segment' and similar phrases.}
    \item \textbf{Three clips}: \texttt{You are given a series of continuous frames divided into 3 segments. Identify and describe the new information appearing in each segment. New information refers to details not discernible from previous frames. This includes human actions, the appearance of new objects, or changes in the scene. For human-related content, provide specific descriptions, such as 'a person talks while looking down', instead of just stating 'talking'. If no humans are present, avoid assuming or creating human actions. Include details of scene changes or new objects that appear. Aim for precision in your descriptions. If no significant actions or new objects are visible, describe any notable camera movements. Avoid using directional terms like 'left' and 'right'. Provide the observations in 3 separate captions divided by a '\#'. Each caption should be detailed, containing approximately five sentences that cover the actions of the main and secondary subjects, any new subjects or objects, and any changes in camera movement. Refrain from using subjective interpretations such as 'indicating' or 'suggesting', and avoid starting phrases like 'as the frames progress'. Directly generate factual and observational captions without introductory phrases like 'Segment 1:' or 'In this/first/second segment'. The captions should be useful for text-to-video generation task. Avoid to generate 'the first/second/third segment' and similar phrases.}
\end{itemize}
We generate
